# Supplementary material for: CellChain: Benchmarking Cross-Scale Evidence Use for Perturbation Reasoning
Source: arXiv:2610.16346 source file (2026-11-16)
Supplement: Supplementary file 1 [file scope_limits.tex]

% \section{Scope and Interpretation}
% \label{app:scope_limits}

% \ours measures prediction changes, not internal reasoning mechanisms. Gene-name masking does not ensure identity anonymity because molecular evidence can retain explicit accessions. Cytokine process annotations are selected through the true stimulus, and the released candidate sets uniquely identify their associated target axes within the cohort; this limits interpretation of both absolute accuracy and process-associated gains as response-based reasoning. Drug histories encode general cell-model sensitivity, and the 240-case cohort was previously inspected for evidence signal, so its results are descriptive rather than untouched-test estimates. The present evaluation does not isolate identity-free Gene prediction, response-derived Cytokine process reasoning, or query-specific Drug integration beyond general sensitivity. Cross-dataset differences, pretrained knowledge, and changes in prompt length or coherence further limit mechanistic attribution.

% The task-specific designs do not separate task characteristics from control-design effects: Gene increments depend on a fixed order, Cytokine Joint redistributes a finite budget, and only Drug tests history assignment. No length-matched or order-matched controls isolate these factors. Endpoint margins do not quantify label uncertainty, and cross-assay alignment does not establish experimental equivalence. Selected cases with limited cellular coverage do not support broad unseen-context generalization. Finally, intervals reflect the fixed model panel under perturbation clustering, without establishing robustness to crossed biological dependencies, model-family composition, or all multiple comparisons.

% The evidence graph provides source-linked organization rather than an independently evaluated graph-reasoning component. Resource coverage does not establish each resource's incremental contribution. Cross-source entity linkage also does not quantify protocol mismatch or its contribution to prediction errors.
